# Supplementary material for: Citation Sentiment Reflects Multiscale Sociocultural Norms
Source: arXiv:2411.09675 ancillary file (2024-12-05)
Supplement: Supplementary file 1 [file Supplement.pdf]

# Supplement: Citation Sentiment Reflects Multiscale Sociocultural Norms

Xiaohuan Xia,<sup>1</sup> Mathieu Ouellet,<sup>2</sup> Shubhankar P. Patankar,<sup>1</sup>

Diana I. Tamir,<sup>3</sup> and Dani S. Bassett<sup>1, 4, 2, 5, 6, 7, 8, \*</sup>

<sup>1</sup>*Department of Bioengineering, University of Pennsylvania, Philadelphia, PA 19104 USA*

<sup>2</sup>*Department of Electrical & Systems Engineering,*

*University of Pennsylvania, Philadelphia, PA 19104 USA*

<sup>3</sup>*Department of Psychology, Princeton University, Princeton, NJ 08544 USA*

<sup>4</sup>*Department of Physics and Astronomy,*

*University of Pennsylvania, Philadelphia, PA 19104 USA*

<sup>5</sup>*Department of Neurology, University of Pennsylvania, Philadelphia, PA 19104 USA*

<sup>6</sup>*Department of Psychiatry, University of Pennsylvania, Philadelphia, PA 19104 USA*

<sup>7</sup>*Santa Fe Institute, Santa Fe, NM 87501 USA*

<sup>8</sup>*Montreal Neurological Institute, McGill University, Montreal, QC H3A 2B4, Canada*

## I. ASSIGNING CITATION SENTIMENT BY LLM

We measure citation sentiment by prompting GPT-3.5-Turbo-1106 with the following system and user prompts:

System Prompt:

For each in-text citation, the rater should measure the sentiment of the citing research toward the cited research (represented as the character U+272A), on a scale of -1 to 1. The rater should assign a positive score (+1) to statements depicting the cited research as positive, corroborative, consistent with, similar to, or in common with the citing research. Conversely, the rater should assign a negative score (-1) to statements depicting the cited research as negative, refuting, inconsistent with, dissimilar to, or different from the citing research. If the statements are neutral or do not belong to the aforementioned categories, then the rater should assign 0 to the statements. When you are given a sentence only answer with the numerical results without explanation.

User Prompt:

The sentence to analyze is: [INSERT: citation sentence.]

The location of U+272A indicates to the model where the citation appears in the sentence. Consider the following sentence as an example: “Lorem ipsum odor amet, consectetur adipiscing elit U+272A.” We choose this Unicode character as it is extremely unlikely to appear in an actual sentence in an article.

### A. Model Finetuning

However, before passing citation sentences to the LLM for sentiment assignment, we first finetune the model on a small dataset of human-annotated examples. As described in the Main text, we obtain annotations from five individuals for 300 citation sentences and split this data into 144 training and 156 validation data points. One of the affordances of fine-tuning LLMs is that we can encourage the model to produce well-formatted outputs. After fine-tuning, GPT-3.5-Turbo-1106 produces less than 0.00004% poorly formatted outputs in

---

\* Corresponding author: dsb@seas.upenn.edu

a dataset with 627108 sentences. We also observe that, compared to the base model and other humans, the outputs of the fine-tuned model show a stronger correlation with human annotators.

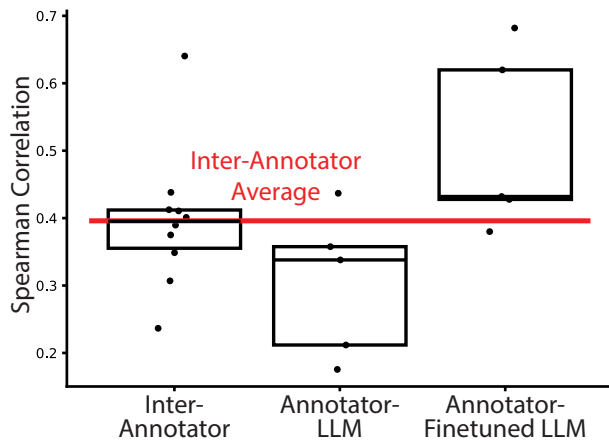

FIG. S1. **Inter-annotator agreement on citation sentences from the validation dataset.** Compared to the base model and other humans, fine-tuned model outputs correlate more with human annotators.

The following are examples of citation sentences labeled by the LLM as being favorable, neutral, and critical:

**Favorable:** “Multiple lines of evidence support the cell-to-cell transfer of insoluble  $\alpha$ Syn.”

**Neutral:** “One of the methods reflecting the interaction of neural activity between brain regions focuses on the functional connectivity among neural networks.”

**Critical:** “Other FDA approved MS therapies, including high potency ocrelizumab, failed to reduce serum levels of IFN $\gamma$  or IL-17.”

## II. BENCHMARK SCORE

We use a base version of GPT-3.5-Turbo-1106 to obtain benchmark scores for different disciplines using the following prompt texts:

System Prompt:

You are a reviewer with expertise in assessing the data sources of research papers. Your task is to determine whether a paper is based on data collected directly by the authors, or from data from other sources, such as using data from another lab, previous research, or relying on computational or theoretical methods. Answer only ‘‘Yes’’ if the authors collected their own data, or only ‘‘No’’ if the data came from external sources, simulations, or purely theoretical origins.

User Prompt:

The paper snippet is: [INSERT: first 10000 tokens of paper text].

We assign a value of 1 to ‘‘Yes’’ and 0 to ‘‘No’’, then calculate the benchmark scores for departments by determining the proportion of 1s among all benchmark labels.

### III. CITATION FREQUENCY

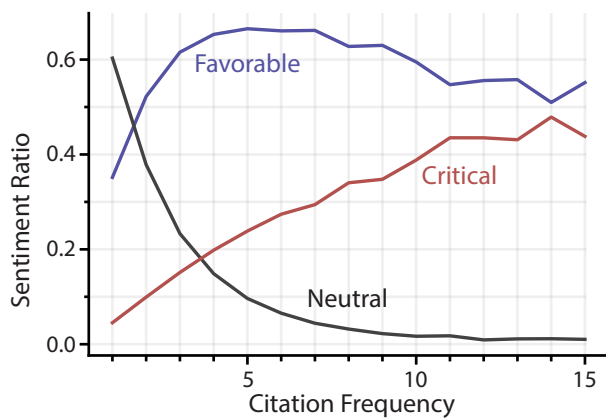

FIG. S2. **Effect of citation frequency on sentiment.** An article can cite another article multiple times. In such instances, we aggregate overall sentiment via the following order of precedence: negative sentiment takes precedence over positive sentiment, and both take precedence over neutral sentiment. This approach reduces multiple citation instances to a single sentiment value. However, the original citation frequency still impacts the overall aggregated sentiment. Therefore, to account for this effect, we explicitly incorporate the number of citations from a citing to a cited work into the null model.

#### IV. EFFECT OF PERCEIVED BRILLIANCE ON CITATION SENTIMENT

The perceived level of brilliance required to operate in a scientific discipline is correlated with its gender ratio [1]. We assess whether such perceptions are also correlated with citation sentiment. We obtain brilliance scores for departments from Muradoglu *et al.* [2] and find that this measure is not significantly related to either favorable or critical citation sentiment.

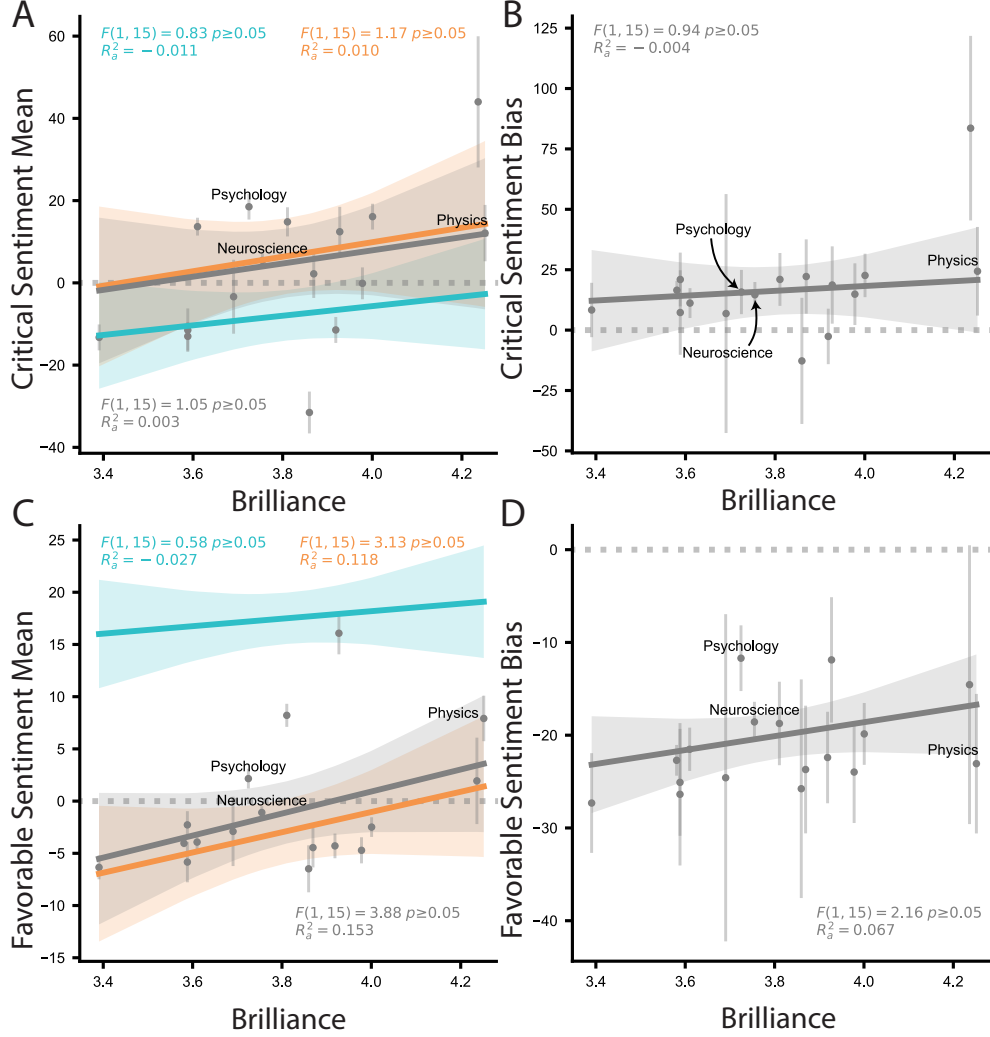

FIG. S3. Citation sentiment as a function of perceived brilliance. (A, B) Mean and bias in critical sentiment as a function of the brilliance score. (C, D) Mean and bias in favorable sentiment as a function of the brilliance score.

## V. LIST OF JOURNALS

TABLE I: The 181 journals included in analyses.

| Journal Title                                                        | JIF  | % OA  | Gold # | Papers |
|----------------------------------------------------------------------|------|-------|--------|--------|
| ACS Chemical Neuroscience                                            | 5    | 13.11 | 251    |        |
| Acta Neuropathologica                                                | 12.7 | 60.92 | 643    |        |
| Acta Neuropathologica Communications                                 | 7.1  | 99.82 | 1445   |        |
| Acta Neuropsychiatrica                                               | 3.8  | 25.98 | 1      |        |
| Alzheimer's & Dementia<br>(Amsterdam, Netherlands)                   | 5.3  | 56.76 | 648    |        |
| Alzheimer's & Dementia<br>(New York, N. Y.)                          | 4.8  | 69.73 | 515    |        |
| Alzheimer's Research & Therapy                                       | 9    | 99.82 | 1405   |        |
| Annals of Clinical and<br>Translational Neurology                    | 5.3  | 69.67 | 1070   |        |
| Annals of Neurology                                                  | 11.2 | 32.6  | 332    |        |
| Annual Review of Neuroscience                                        | 13.9 | 0     | 1      |        |
| ASN Neuro                                                            | 4.7  | 94.5  | 377    |        |
| Behavioral and Brain Functions                                       | 5.1  | 100   | 527    |        |
| Biological Psychiatry                                                | 10.6 | 33.46 | 158    |        |
| Biological Psychiatry:<br>Cognitive Neuroscience<br>and Neuroimaging | 5.9  | 28.06 | 42     |        |
| Bipolar Disorders                                                    | 5.9  | 20.33 | 40     |        |
| Brain: A Journal of Neurology                                        | 14.5 | 45.12 | 1190   |        |
| Brain and Behavior                                                   | 3.1  | 69.26 | 1891   |        |
| Brain Communications                                                 | 4.8  | 93.5  | 1041   |        |
| Brain Connectivity                                                   | 3.4  | 11.41 | 39     |        |
| Brain Pathology (Zurich, Switzerland)                                | 6.4  | 52.89 | 264    |        |
| Brain Research Bulletin                                              | 3.8  | 14.76 | 27     |        |
| Brain Sciences                                                       | 3.3  | 99.39 | 5303   |        |
| Brain Stimulation                                                    | 7.7  | 94.43 | 126    |        |
| Brain Structure & Function                                           | 3.1  | 39.15 | 585    |        |
| Brain, Behavior, and Immunity                                        | 15.1 | 32.18 | 175    |        |
| Cellular and Molecular Neurobiology                                  | 4    | 12.72 | 139    |        |
| Cephalalgia                                                          | 4.9  | 22.57 | 148    |        |
| Cerebellum (London, England)                                         | 3.5  | 27.34 | 173    |        |
| Cerebral Cortex (New York, N.Y. : 1991)                              | 3.7  | 26.84 | 1188   |        |
| Chemical Senses                                                      | 4.2  | 15.09 | 47     |        |
| Clinical Autonomic Research                                          | 5.8  | 24.44 | 62     |        |
| Clinical Neurophysiology                                             | 4.7  | 27.98 | 78     |        |
| Clinical Psychopharmacology<br>and Neuroscience                      | 3.2  | 100   | 473    |        |
| Clocks & Sleep                                                       | 3.1  | 99.26 | 152    |        |
| CNS & Neurological Disorders - Drug Targets                          | 3    | 1.9   | 11     |        |
| CNS Neuroscience & Therapeutics                                      | 5.5  | 62.96 | 811    |        |
| Cognitive Computation                                                | 5.4  | 16    | 19     |        |
| Cognitive Neurodynamics                                              | 3.7  | 12.15 | 64     |        |
| Cortex                                                               | 3.6  | 32.6  | 172    |        |
| Current Neurology and<br>Neuroscience Reports                        | 5.6  | 14.88 | 5      |        |
| Current Neuropharmacology                                            | 5.3  | 5.23  | 1105   |        |
| Current Opinion in Behavioral Sciences                               | 5    | 33.95 | 25     |        |
| Current Opinion in Neurobiology                                      | 5.7  | 41.24 | 65     |        |
| Current Opinion in Neurology                                         | 4.8  | 10.17 | 60     |        |
| Developmental Cognitive Neuroscience                                 | 4.7  | 97.25 | 980    |        |
| Developmental Neurobiology                                           | 3    | 25.93 | 52     |        |
| Dialogues in Clinical Neuroscience                                   | 8.3  | 72.22 | 567    |        |
| eNeuro                                                               | 3.4  | 97.68 | 2307   |        |
| Epilepsia                                                            | 5.6  | 27.45 | 259    |        |
| Epilepsia Open                                                       | 3    | 66.26 | 425    |        |

TABLE I: The 181 journals included in analyses.

| Journal Title                                              | JIF  | % OA Gold | # Papers |
|------------------------------------------------------------|------|-----------|----------|
| European Journal of Neurology                              | 5.1  | 28.35     | 232      |
| European Journal of Pain<br>(London, England)              | 3.6  | 32.08     | 120      |
| European Neuropsychopharmacology                           | 5.6  | 25.21     | 35       |
| Experimental Neurology                                     | 5.3  | 18.8      | 73       |
| Fluids and Barriers of the CNS                             | 7.3  | 99.56     | 540      |
| Frontiers in Aging Neuroscience                            | 4.8  | 99.41     | 5116     |
| Frontiers in Cellular Neuroscience                         | 5.3  | 99.44     | 4741     |
| Frontiers in Computational Neuroscience                    | 3.2  | 99.06     | 1404     |
| Frontiers in Integrative Neuroscience                      | 3.5  | 99.17     | 843      |
| Frontiers in Molecular Neuroscience                        | 4.8  | 99.69     | 3245     |
| Frontiers in Neural Circuits                               | 3.5  | 99.45     | 1370     |
| Frontiers in Neuroendocrinology                            | 7.4  | 25.19     | 11       |
| Frontiers in Neuroinformatics                              | 3.5  | 99.63     | 682      |
| Frontiers in Neurology                                     | 3.4  | 99.46     | 8631     |
| Frontiers in Neurorobotics                                 | 3.1  | 99.82     | 637      |
| Frontiers in Neuroscience                                  | 4.3  | 99.26     | 10364    |
| Frontiers in Synaptic Neuroscience                         | 3.7  | 100       | 445      |
| Frontiers in Systems Neuroscience                          | 3    | 99.24     | 1393     |
| Glia                                                       | 6.2  | 28.49     | 245      |
| Hippocampus                                                | 3.5  | 18.49     | 110      |
| Human Brain Mapping                                        | 4.8  | 67.82     | 1702     |
| International Journal of Psychophysiology                  | 3    | 19.25     | 15       |
| International Journal of<br>Tryptophan Research            | 4.4  | 98        | 124      |
| Journal of Alzheimer's Disease                             | 4    | 17.88     | 15       |
| Journal of Cerebral Blood Flow<br>and Metabolism           | 6.3  | 24.73     | 379      |
| Journal of Cognitive Neuroscience                          | 3.2  | 9.91      | 16       |
| Journal of Huntington's Disease                            | 3.1  | 32.08     | 1        |
| Journal of Molecular Neuroscience                          | 3.1  | 10.3      | 158      |
| Journal of Neural Engineering                              | 4    | 30.11     | 86       |
| Journal of Neural Transmission<br>(Vienna, Austria : 1996) | 3.3  | 45.29     | 347      |
| Journal of Neurochemistry                                  | 4.7  | 19.3      | 201      |
| Journal of Neurodevelopmental Disorders                    | 4.9  | 100       | 516      |
| Journal of Neuroendocrinology                              | 3.2  | 20.27     | 99       |
| Journal of Neuroengineering<br>and Rehabilitation          | 5.1  | 99.79     | 1597     |
| Journal of Neuroimmune Pharmacology                        | 6.2  | 12.58     | 101      |
| Journal of Neuroimmunology                                 | 3.3  | 10.76     | 43       |
| Journal of Neuroinflammation                               | 9.3  | 100       | 3673     |
| Journal of Neuromuscular Diseases                          | 3.3  | 36.57     | 27       |
| Journal of Neuropathology<br>and Experimental Neurology    | 3.2  | 16.11     | 100      |
| Journal of Neuroscience Methods                            | 3    | 30.4      | 106      |
| Journal of Neuroscience Research                           | 4.2  | 14.34     | 96       |
| Journal of Neurotrauma                                     | 4.2  | 13.52     | 181      |
| Journal of Neurovirology                                   | 3.2  | 13.55     | 120      |
| Journal of Parkinson's Disease                             | 5.2  | 41.22     | 6        |
| Journal of Pineal Research                                 | 10.3 | 19.34     | 25       |
| Journal of Psychiatry & Neuroscience                       | 4.3  | 100       | 121      |
| Journal of Psychopharmacology<br>(Oxford, England)         | 4.1  | 30.53     | 240      |
| Journal of Sleep Research                                  | 4.4  | 23.34     | 94       |
| Journal of the Neurological Sciences                       | 4.4  | 14.34     | 67       |
| Journal of the Peripheral Nervous System                   | 3.8  | 20.93     | 20       |
| Metabolic Brain Disease                                    | 3.6  | 4.54      | 89       |
| Molecular and Cellular Neurosciences                       | 3.5  | 24.29     | 42       |
| Molecular Autism                                           | 6.2  | 99.53     | 657      |

TABLE I: The 181 journals included in analyses.

| Journal Title                                            | JIF  | % OA Gold | # Papers |
|----------------------------------------------------------|------|-----------|----------|
| Molecular Brain                                          | 3.6  | 99.77     | 1024     |
| Molecular Neurobiology                                   | 5.1  | 21.12     | 740      |
| Molecular Neurodegeneration                              | 15.1 | 100       | 1005     |
| Molecular Pain                                           | 3.3  | 94.5      | 1301     |
| Molecular Psychiatry                                     | 11   | 45.71     | 1697     |
| Multiple Sclerosis<br>(Houndmills, Basingstoke, England) | 5.8  | 21.94     | 339      |
| Muscle & Nerve                                           | 3.4  | 14.48     | 100      |
| Nature Aging                                             | 16.6 | 19.53     | 44       |
| Nature and Science of Sleep                              | 3.4  | 96.55     | 471      |
| Nature Human Behaviour                                   | 29.9 | 9.69      | 98       |
| Nature Neuroscience                                      | 25   | 10.39     | 1384     |
| Nature Reviews: Neurology                                | 38.1 | 4.17      | 31       |
| Nature Reviews: Neuroscience                             | 34.7 | 2.11      | 8        |
| Network: Computation in Neural Systems                   | 7.8  | 4.76      | 1        |
| Network Neuroscience<br>(Cambridge, Mass.)               | 4.7  | 97.96     | 313      |
| Neural Development                                       | 3.6  | 100       | 301      |
| Neural Networks                                          | 7.8  | 16.76     | 9        |
| Neural Plasticity                                        | 3.1  | 99.32     | 1595     |
| Neural Regeneration Research                             | 6.1  | 96        | 1492     |
| Neuro-Degenerative Diseases                              | 3    | 17.19     | 8        |
| Neurobiology of Aging                                    | 4.2  | 29.95     | 194      |
| Neurobiology of Disease                                  | 6.1  | 96.26     | 291      |
| Neurobiology of Language<br>(Cambridge, Mass.)           | 3.2  | 100       | 95       |
| Neurobiology of Stress                                   | 5    | 96.8      | 510      |
| Neurochemical Research                                   | 4.4  | 11.78     | 228      |
| Neurochemistry International                             | 4.2  | 16.46     | 19       |
| Neuroendocrinology                                       | 4.1  | 17.38     | 10       |
| Neurogastroenterology and Motility                       | 3.5  | 15.19     | 38       |
| NeuroImage                                               | 5.7  | 96.27     | 1561     |
| NeuroImage: Clinical                                     | 4.2  | 99.65     | 3364     |
| Neuroinformatics                                         | 3    | 37.71     | 117      |
| Neurological Sciences                                    | 3.3  | 16.84     | 430      |
| Neurology(R) Neuroimmunology<br>& Neuroinflammation      | 8.8  | 99.01     | 793      |
| Neuromolecular Medicine                                  | 3.5  | 13.5      | 58       |
| Neuron                                                   | 16.2 | 74.45     | 378      |
| Neuropathology and<br>Applied Neurobiology               | 5    | 46.15     | 128      |
| Neuropharmacology                                        | 4.7  | 22.03     | 103      |
| Neurophotonics                                           | 5.3  | 98.69     | 293      |
| Neurophysiologie Clinique<br>(Clinical Neurophysiology)  | 3    | 28.57     | 2        |
| Neuropsychobiology                                       | 3.2  | 9.92      | 6        |
| Neuropsychology review                                   | 5.8  | 28.68     | 69       |
| Neuropsychopharmacology                                  | 7.6  | 29.78     | 544      |
| Neuroscience                                             | 3.3  | 17.06     | 133      |
| Neuroscience and Biobehavioral Reviews                   | 8.2  | 28.33     | 96       |
| Neuroscience Bulletin                                    | 5.6  | 26.94     | 164      |
| Neuroscience Insights                                    | 3.6  | 92.59     | 62       |
| Neurotherapeutics                                        | 5.7  | 29.75     | 259      |
| Neurotoxicity Research                                   | 3.7  | 7.74      | 151      |
| Neurotoxicology                                          | 3.4  | 17.82     | 11       |
| NPJ Parkinson's Disease                                  | 8.7  | 99.69     | 565      |
| NPJ Science of Learning                                  | 4.2  | 100       | 128      |
| Nutritional Neuroscience                                 | 3.6  | 8.51      | 6        |
| Pain                                                     | 7.4  | 17.41     | 414      |
| Pain Reports                                             | 4.8  | 99.1      | 318      |

TABLE I: The 181 journals included in analyses.

| Journal Title                                                   | JIF        | % OA         | Gold #        | Papers |
|-----------------------------------------------------------------|------------|--------------|---------------|--------|
| Pharmacology, Biochemistry, and Behavior                        | 3.6        | 16.49        | 11            |        |
| Progress in Neuro-Psychopharmacology<br>& Biological Psychiatry | 5.6        | 16.76        | 24            |        |
| Progress in Neurobiology                                        | 6.7        | 44.22        | 41            |        |
| Psychiatry and Clinical Neurosciences                           | 11.9       | 29.76        | 35            |        |
| Psychoneuroendocrinology                                        | 3.7        | 27.17        | 69            |        |
| Psychopharmacology                                              | 3.4        | 21.66        | 678           |        |
| Psychophysiology                                                | 3.7        | 25.99        | 107           |        |
| Purinergic Signalling                                           | 3.5        | 34.08        | 188           |        |
| Seizure                                                         | 3          | 61.9         | 29            |        |
| Sleep                                                           | 5.6        | 24.05        | 202           |        |
| Sleep Medicine Reviews                                          | 10.5       | 21.25        | 11            |        |
| Social Cognitive and<br>Affective Neuroscience                  | 4.2        | 95.97        | 828           |        |
| The European Journal of Neuroscience                            | 3.4        | 25.18        | 480           |        |
| The International Journal of<br>Neuropsychopharmacology         | 4.8        | 91.11        | 768           |        |
| The Journal of Headache and Pain                                | 7.4        | 99.52        | 1476          |        |
| The Journal of Neuroscience                                     | 5.3        | 60.25        | 629           |        |
| The Journal of Pain                                             | 4          | 16.58        | 23            |        |
| The Journal of Physiology                                       | 5.5        | 32.82        | 322           |        |
| The Neuroscientist                                              | 5.6        | 17.24        | 53            |        |
| Translational Neurodegeneration                                 | 12.6       | 100          | 393           |        |
| Translational Stroke Research                                   | 6.9        | 26.83        | 147           |        |
| Trends in Cognitive Sciences                                    | 19.9       | 29.17        | 51            |        |
| Trends in Neuroscience and Education                            | 3.3        | 26.98        | 8             |        |
| Trends in Neurosciences                                         | 15.9       | 30.91        | 53            |        |
| <b>Average</b>                                                  | <b>6.0</b> | <b>47.51</b> | <b>601.7</b>  |        |
| <b>Standard Deviation</b>                                       | <b>5.0</b> | <b>35.51</b> | <b>1269.1</b> |        |

## VI. LIST OF DEPARTMENTS

TABLE II. 28 departments.

| Department<br>(Alternative<br>Search Name)   | Number of<br>Last Authors | Number of<br>Last Author Papers | Number of<br>First Authors | Number of<br>First Author Papers |
|----------------------------------------------|---------------------------|---------------------------------|----------------------------|----------------------------------|
| Anatomy                                      | 1145                      | 2084                            | 1672                       | 1949                             |
| Behavior                                     | 1830                      | 2991                            | 2197                       | 2507                             |
| Biochemistry                                 | 840                       | 1292                            | 1062                       | 1183                             |
| Biology                                      | 5587                      | 9381                            | 7762                       | 8777                             |
| Biomedical                                   | 3530                      | 6260                            | 4744                       | 5556                             |
| Cell                                         | 2756                      | 4491                            | 3487                       | 3850                             |
| Compute<br>(Computational)                   | 1133                      | 1940                            | 1743                       | 2059                             |
| Engineering                                  | 3309                      | 5798                            | 4922                       | 5718                             |
| Genetics                                     | 1549                      | 2506                            | 2070                       | 2326                             |
| Imaging                                      | 2386                      | 5224                            | 3773                       | 4805                             |
| Information                                  | 557                       | 933                             | 929                        | 1127                             |
| Mathematics                                  | 239                       | 313                             | 321                        | 355                              |
| Medical<br>(Medicine)                        | 25979                     | 47156                           | 36983                      | 45746                            |
| Mental                                       | 4199                      | 7409                            | 6005                       | 7092                             |
| Molecular                                    | 3124                      | 5285                            | 4146                       | 4743                             |
| Neurology<br>(Neurological)                  | 8396                      | 17291                           | 12568                      | 16021                            |
| Neuroscience                                 | 10229                     | 19974                           | 14899                      | 18047                            |
| Ophthalmology                                | 577                       | 885                             | 704                        | 793                              |
| Pathology                                    | 1166                      | 1962                            | 1490                       | 1764                             |
| Pharmacy,<br>Pharmacology,<br>Pharmaceutical | 3553                      | 5822                            | 4703                       | 5433                             |
| Physics<br>(Physical Science)                | 955                       | 1599                            | 1315                       | 1487                             |
| Physiology<br>(Physiological)                | 3440                      | 6283                            | 4958                       | 5749                             |
| Psychiatry                                   | 4439                      | 8581                            | 6013                       | 7463                             |
| Psychology<br>(Psychological)                | 4790                      | 8835                            | 7303                       | 8836                             |
| Radiology                                    | 1584                      | 3158                            | 2223                       | 2887                             |
| Statistics                                   | 346                       | 485                             | 389                        | 437                              |
| Surgery                                      | 3093                      | 5126                            | 4004                       | 4733                             |
| Therapy                                      | 1132                      | 1909                            | 1589                       | 1908                             |

## VII. LIST OF COUNTRIES AND REGIONS

TABLE III. 23 countries and regions.

| Country/Region      | Power Distance | Individualism | Number of Last Authors | Number of Last Author Papers | Number of First Authors | Number of First Author Papers |
|---------------------|----------------|---------------|------------------------|------------------------------|-------------------------|-------------------------------|
| Australia (AU)      | 38             | 90            | 1472                   | 2639                         | 2137                    | 2574                          |
| Austria (AT)        | 11             | 55            | 421                    | 858                          | 692                     | 909                           |
| Belgium (BE)        | 65             | 75            | 489                    | 999                          | 876                     | 1063                          |
| Canada (CA)         | 39             | 80            | 2025                   | 4160                         | 3352                    | 4084                          |
| China (CN)          | 80             | 20            | 8163                   | 16197                        | 12523                   | 17040                         |
| Denmark (DK)        | 18             | 74            | 523                    | 944                          | 730                     | 887                           |
| Finland (FI)        | 33             | 63            | 324                    | 607                          | 500                     | 605                           |
| France (FR)         | 68             | 71            | 1697                   | 2694                         | 2345                    | 2711                          |
| Germany (DE)        | 35             | 67            | 3634                   | 7216                         | 5974                    | 7355                          |
| Ireland (IE)        | 28             | 70            | 185                    | 334                          | 288                     | 326                           |
| Israel (IL)         | 13             | 54            | 422                    | 722                          | 639                     | 739                           |
| Italy (IT)          | 50             | 76            | 2576                   | 5064                         | 3818                    | 5255                          |
| Japan (JP)          | 54             | 46            | 1622                   | 3257                         | 2769                    | 3375                          |
| Netherlands (NL)    | 38             | 80            | 1621                   | 3126                         | 2682                    | 3277                          |
| Norway (NO)         | 31             | 69            | 379                    | 740                          | 547                     | 699                           |
| Poland (PL)         | 68             | 60            | 582                    | 983                          | 795                     | 1041                          |
| South Korea (KR)    | 60             | 18            | 982                    | 1919                         | 1541                    | 1955                          |
| Spain (ES)          | 57             | 51            | 1429                   | 2310                         | 2005                    | 2411                          |
| Sweden (SE)         | 31             | 71            | 852                    | 1776                         | 1339                    | 1717                          |
| Switzerland (CH)    | 34             | 68            | 1104                   | 2025                         | 1658                    | 2054                          |
| Taiwan (TW)         | 58             | 17            | 532                    | 897                          | 766                     | 925                           |
| United Kingdom (GB) | 35             | 89            | 4532                   | 9695                         | 7334                    | 9465                          |
| United States (US)  | 40             | 91            | 14518                  | 26111                        | 20984                   | 25307                         |

- 
- [1] S. J. Leslie, A. Cimpian, M. Meyer, and E. Freeland, Expectations of brilliance underlie gender distributions across academic disciplines, *Science* **347**, 262 (2015).
- [2] M. Muradoglu, Z. Horne, M. D. Hammond, S.-J. Leslie, and A. Cimpian, Women—particularly underrepresented minority women—and early-career academics feel like impostors in fields that value brilliance, *Journal of Educational Psychology* **114**, 1086 (2022).
